# Supplementary material for: Leveraging Verifier-Based Reinforcement Learning in Image Editing
Source: arXiv:2604.27505 source file (2026-05-20)
Supplement: Supplementary file 1 [file appendix.tex]

\section{Hello World}
%\subsection{Hello World}
